# Supplementary material for: Spatial Entropy as an Inductive Bias for Vision Transformers
Source: arXiv:2206.04636 source file (2023-03-14)
Supplement: Supplementary file 1 [file in100_supplementary.tex]

\begin{table}[t]
\vspace{2mm}
\setlength{\tabcolsep}{1.0pt}
%\caption{(a) Out-of-distribution testing robustness. (b) A  comparison of the segmentation properties of the attention maps on PASCAL VOC-12. }
%\label{tab:robustness_results}
%\label{tab:PASCAL-VOC}
\small
    \begin{minipage}[t]{.5\textwidth}
        \caption{IN-100 experiments with different VTs. For each tested VT, we plug SAR on the publicly available code of the corresponding baseline and we use the suggested hyperparameter values for training. All the results are obtained using 100 training epochs.}
        \label{tab:imagenet-100}
        \centering
        \begin{tabular}{ll}
            \toprule
            \textbf{Model} & \textbf{Top-1 Acc.}  \\
            \midrule
            ViT-S/16~\citep{ViT}  & 74.22 \\
            \rowcolor{Light}ViT-S/16 + SAR & \textbf{76.72}   \posimprov{2.5} \\
            \midrule
            T2T-ViT-14~\citep{T2T} & 82.42   \\
            \rowcolor{Light}T2T-ViT-14 + SAR & \textbf{83.96} \posimprov{1.54} \\
            \midrule
            PVT-Small~\citep{PVT} & 76.57 \\
            \rowcolor{Light}PVT-Small + SAR  & \textbf{77.78} \posimprov{1.21} \\
            \midrule
            CvT-13~\citep{CvT} & 83.38 \\
            \rowcolor{Light}CvT-13 + SAR  & \textbf{85.20} \posimprov{1.82} \\
            \bottomrule
        \end{tabular}
    \end{minipage}
    \hfill
    \begin{minipage}[t]{.45\textwidth}
    %\captionsetup{labelformat=empty} 
    \caption{IN-100 experiments with different sampling ratio strategies.}
    \label{tab:sampling_ratio_in100}
    \centering
        \begin{tabular}{lll}
        \toprule
        \textbf{Sampling Ratio} & \textbf{ViT-S/16} & \textbf{ViT-S/16+SAR}\\ 
        \midrule
        0.25 & 21.66 & 29.06 \posimprov{7.4} \\
        0.50 & 29.86 & 38.02 \posimprov{8.16} \\
        0.75 & 35.62 & 46.12 \posimprov{10.5} \\
        1.00 & 74.22 & 76.72 \posimprov{2.5} \\
        \bottomrule
        \end{tabular}
    \end{minipage}
\end{table}
